# Supplementary material for: MROVSeg: Breaking the Resolution Curse of Vision-Language Models in Open-Vocabulary Image Segmentation
Source: arXiv:2408.14776 source file (2024-11-27)
Supplement: Supplementary file 1 [file sec_X_supp.tex]

\setcounter{section}{0}
\vspace{20pt}

% \noindent \textbf{\Large Appendix}

\section{Overview}
In the supplementary material for MROVSeg, we provide implementation detail (Sec. \ref{sec:supp_implementation}), qualitative results (Sec. \ref{sec:qualitative_results}), and limitation and discussion (Sec. \ref{sec:limitation and discussion}).

\section{Implementation Detail}
\label{sec:supp_implementation}
\subsection{Training Detail}
During the training, we follow common practices~\cite{mask2former,san} to use AdamW optimizer with a base learning rate of $2e-4$ with poly decay schedule power $0.9$ to train the model, and the weight decay is set to $1e-4$. We use the same data augmentation strategies as in~\cite{san,fcclip,ovseg} for training, i.e., all training images firstly are randomly resized to $[0.5, 2.0]\times$ of its
original resolution, then are randomly cropped into the resolution of $640^2$. And for fair comparison, the test-time argumentation is not used. 

\subsection{Multi-grained Masked Attention}
As introduced in Sec. 3.6, we enable the $\mathbf{X}_{\texttt{prop}}$ by perform masked cross attention with multi-resolution CLIP visual tokens. We show the pseudo code in Algorithm \ref{alg:code}. During the inference, denote the number of CLIP token as $N$, the number of CLIP high-resolution token $4N$, the number of query token as  $N_{\texttt{prop}}$, then the time complexity of the cross attention implementation is $\mathcal{O}(5N^2 +20N_{\texttt{query}}N)$.

\subsection{Text Prompt Templates}
Recent works in open-vocabulary image segmentation~\cite{san,maftp} have proven that prompt engineering is useful for CLIP text encoder. In default settings, we follow common practices~\cite{san,odise,maftp,catseg} to generate augmented class description from VILD~\cite{clip} templates as in~\ref{tab:text_template} for CLIP text encoder. We average the text embedding of all descriptions as the class text feature.
\subsection{Model Parameters}
Since MROVSeg is intermixed with various well-established models, we list the parameters of the modules we introduced in~\cref{tab:param}.
\begin{algorithm}[t]
\caption{Pseudocode of Multi-grained Masked Attention in Pytorch-like style.}
\label{alg:code}
\definecolor{codeblue}{rgb}{0.25,0.5,0.5}
\lstset{
  backgroundcolor=\color{white},
  basicstyle=\fontsize{7.2pt}{7.2pt}\ttfamily\selectfont,
  columns=fullflexible,
  breaklines=true,
  captionpos=b,
  commentstyle=\fontsize{7.2pt}{7.2pt}\color{codeblue},
  keywordstyle=\fontsize{7.2pt}{7.2pt},
%  frame=tb,
}
\begin{lstlisting}[language=python]
# visual_tokens: multi-resolution CLIP  visual token with shape (5L, N, C)
# M_local: local attention mask with shape [4L,N,C]
# M_global: global attention mask with shape [L,N,C]
# X_prop: [CLS] token with position embedding
M = torch.cat([M_global, M_local], dim=0)
# load frozen VLM layers
for layer in cross_attn_layers:    
    X_prop = layer(X_prop,visual_tokens,attn_mask=M)
visual_embedding = matmul(X_prop, W_proj)
logits = bmm(visual_embedding, text_embedding.T())

\end{lstlisting}
\end{algorithm}
\begin{table}[t]
    \centering
        \caption{Text templates used for generating class sentences as the input of CLIP text encoder.}
    \begin{tabular}{l}
    \hline
    “a photo of a \{\}.”,\\
“This is a photo of a \{\}”,\\
“There is a \{\} in the scene”,\\
“There is the \{\} in the scene”,\\
“a photo of a \{\} in the scene”,\\
“a photo of a small \{\}.”,\\
“a photo of a medium \{\}.”,\\
“a photo of a large \{\}.”,\\
“This is a photo of a small \{\}.”,\\
“This is a photo of a medium \{\}.”,\\
“This is a photo of a large \{\}.”,\\
“There is a small \{\} in the scene.”,\\
“There is a medium \{\} in the scene.”,\\
“There is a large \{\} in the scene.”,\\
\hline
    \end{tabular}

    \label{tab:text_template}
\end{table}

\section{Qualitative Results}
\label{sec:qualitative_results}
In this section, we provide the segmentation results on COCO-Stuff \textit{val}~\cite{coco-stuff} (close-vocabulary setting), ADE~\cite{ade} and Pascal Context~\cite{pc} (open-vocabulary setting).

\subsection{Open-Vocabulary Panoptic Segmentation}
We show the qualitative results of open-vocabulary panoptic segmentation with ADE~\cite{ade} benckmark in~\cref{fig:panop_ade}. MROVSeg is able to produce accurate results even in complex scenes.

\subsection{Open-vocabulary Semantic Segmentation}
We provide more qualitative comparison of our method MROVSeg with state-of-the-art methods SAN~\cite{san} and EBSeg~\cite{ebseg} in Fig.\ref{fig:qualitative_comparison}. We observe that MROVSeg can handle complex scenarios while preserving spatial details (object boundaries) and extract global context effectively.
\begin{table}[t]
    \centering
        \caption{Text templates used for generating class sentences as the input of CLIP text encoder.}
    \begin{tabular}{c|cc}
    \toprule
Status & Module & \# Param \\ \hline\hline
\multirow{6}{*}{Trainable} & Query \& Positional Embedding &    1.95M\\
 & ViT Blocks & 40.6M \\
 & MRF Modules &  5.4M\\
 & Hierarchical Mask Decoding & 6.9M\\
 & Decoupled Attention Decoding& 2.0M\\
 & Total &  56.8M \\
 \hline
Frozen & \multicolumn{2}{c}{105.3M}  \\
\hline
Total & \multicolumn{2}{c}{162.1M} \\ 
\bottomrule
    \end{tabular}

    \label{tab:param}
\end{table}

\subsection{COCO}

We visualize the closed-vocabulary semantic predictions of COCO-Stuff~\cite{coco-stuff}. As shown in Fig.\ref{fig:qualitative_coco}, our method is able to handle complex scenarios and provide precise mask predictions. However, as the labels exist semantically containment relationships,  our model struggles to distinguish the regions with similar semantics. For instance, the model cannot find out the \textit{donut} out of the \textit{food-other} in fifth row of Fig.\ref{fig:qualitative_coco}(b).

\subsection{ADE}

We visualize the open-vocabulary semantic segmentation predctions of MROVSeg on ADE~\cite{ade} dataset with 150 and 847 categories benchmark respectively. As the result, we find MROVSeg can segment and identify the novel classes that only appear in 847-class annotations. As illustrated in Fig.\ref{fig:qualitative_ade}, the model is able to segment and recognize \textit{phone booth} and \textit{snow} in (b) and (c) of Fig.\ref{fig:qualitative_ade} respectively.

\subsection{Pascal Context}

The qualitative results of segmentation performance of MROVSeg for 59 and 459 semantic categories on Pascal Context~\cite{pc} dataset are shown in Fig.\ref{fig:qualitative_pc}. Note that MROVSeg is able to segment small objects (such as the video camera in Fig.\ref{fig:qualitative_pc}(c)), which is benefit from the high resolution VLM features and strong local contexts.

\section{Disucssion}
\label{sec:limitation and discussion}

In this section, we further discuss the limitation, future work and potential negtive impact of MROVSeg.

\subsection{Limitation and Future Work}
Due to computational constraints and for fair performance comparison, we conduct our experiments solely based on the CLIP~\cite{clip} model. Other vision-language models, such as ALIGN~\cite{align}, should also be relevant to this work. 

This work involves tuning pretrained Vision-Language Models (VLMs) in a parameter-efficient manner, while pretrained VLMs often contain a large number of parameters, which significantly impacts the efficiency of segmentation. Our method requires the use of a sliding window to repeatedly sample the same image multiple times during the inference, which, though affordable (demonstrated in Sec. 4.3), is also computationally unfriendly. 

As shown in the Fig.\ref{fig:qualitative_coco}(b), MROVSeg struggles to distinguish and process semantics with containment relationships, often leading to inaccurate recognition. For future work, introducing semantic priors based on category names is an promising direction to solve this issue. The datasets used in this work suffer from imprecise semantic mask annotations (as illustrated in Fig.\ref{fig:qualitative_pc}(d), the cups on the table are not annotated), which may affect the real running performance of the model. Additionally, the evaluation method for open-vocabulary semantic segmentation has inherent ambiguities as shown in the Fig.\ref{fig:qualitative_pc}(c). The \textit{ground} mask is also reasonable to be classified to \textit{road} as a truck drving on it. Recently, there have been some studies (such as ~\cite{mess}) exploring the performance of open vocabulary semantic segmentation models across a wider range of categories and more specialized data. Thus, investigating more reasonable evaluation methods for open-vocabulary semantic segmentation is also a focus for future work.

\subsection{Dataset usage}
This work involves training segmentation models on public datasets(COCO~\cite{coco}, VOC~\cite{voc}, and ADE~\cite{ade}). These datasets may contain personally identifiable information (such as facial characteristics), but they were responsibly collected and used. These datasets have benefited the image segmentation community for years.

\subsection{Potential Negtive Impact}
This work expands the scope of open-vocabulary semantic segmentation methods, offering significant advantages in areas like healthcare and autonomous driving. However, there is potential for misuse in applications such as surveillance, a common issue in most semantic segmentation research. Implementing regulatory measures to control the application of these algorithms might be an effective solution.
\clearpage
\begin{figure*}[t]
    \centering
    \includegraphics[width=0.97\linewidth]{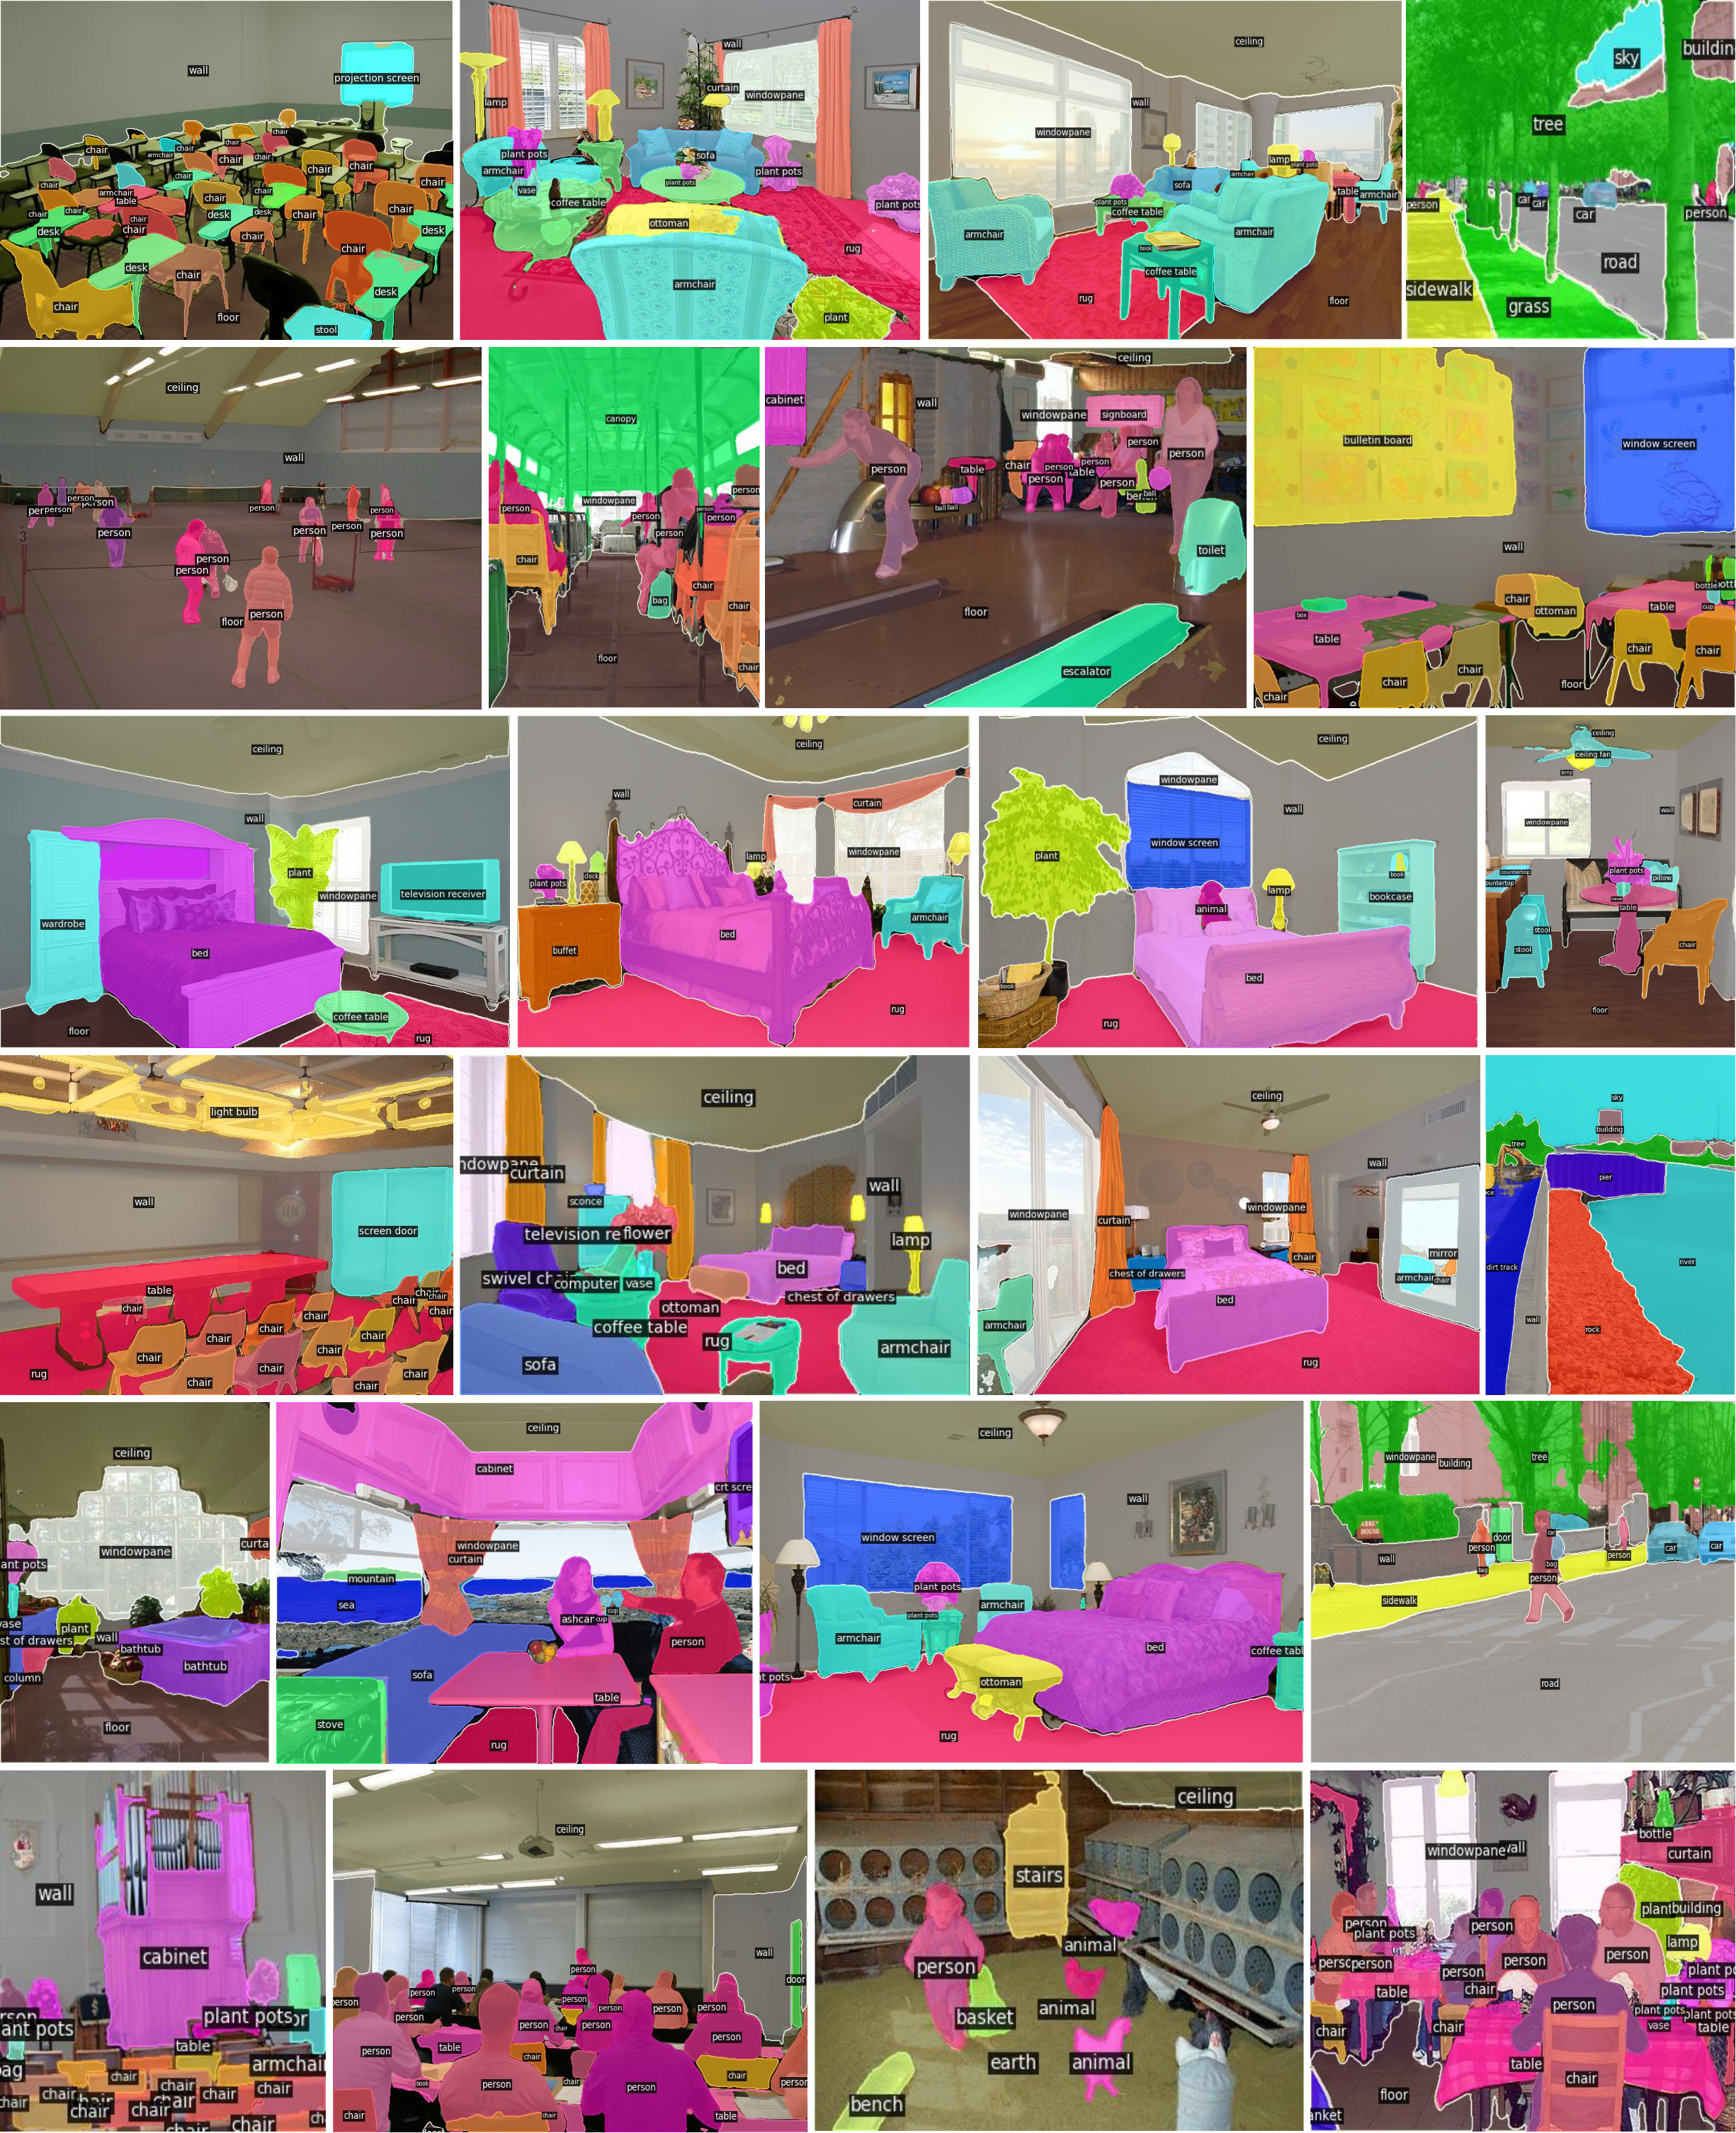}
    \caption{Visualization of panoptic segmentation results on ADE20k~\cite{ade}.}
    \label{fig:panop_ade}
\end{figure*}

\begin{figure*}[t]
  \centering
    % \fbox{\rule{0pt}{2in} \rule{.9\linewidth}{0pt}}
    \includegraphics[width=0.97\linewidth]{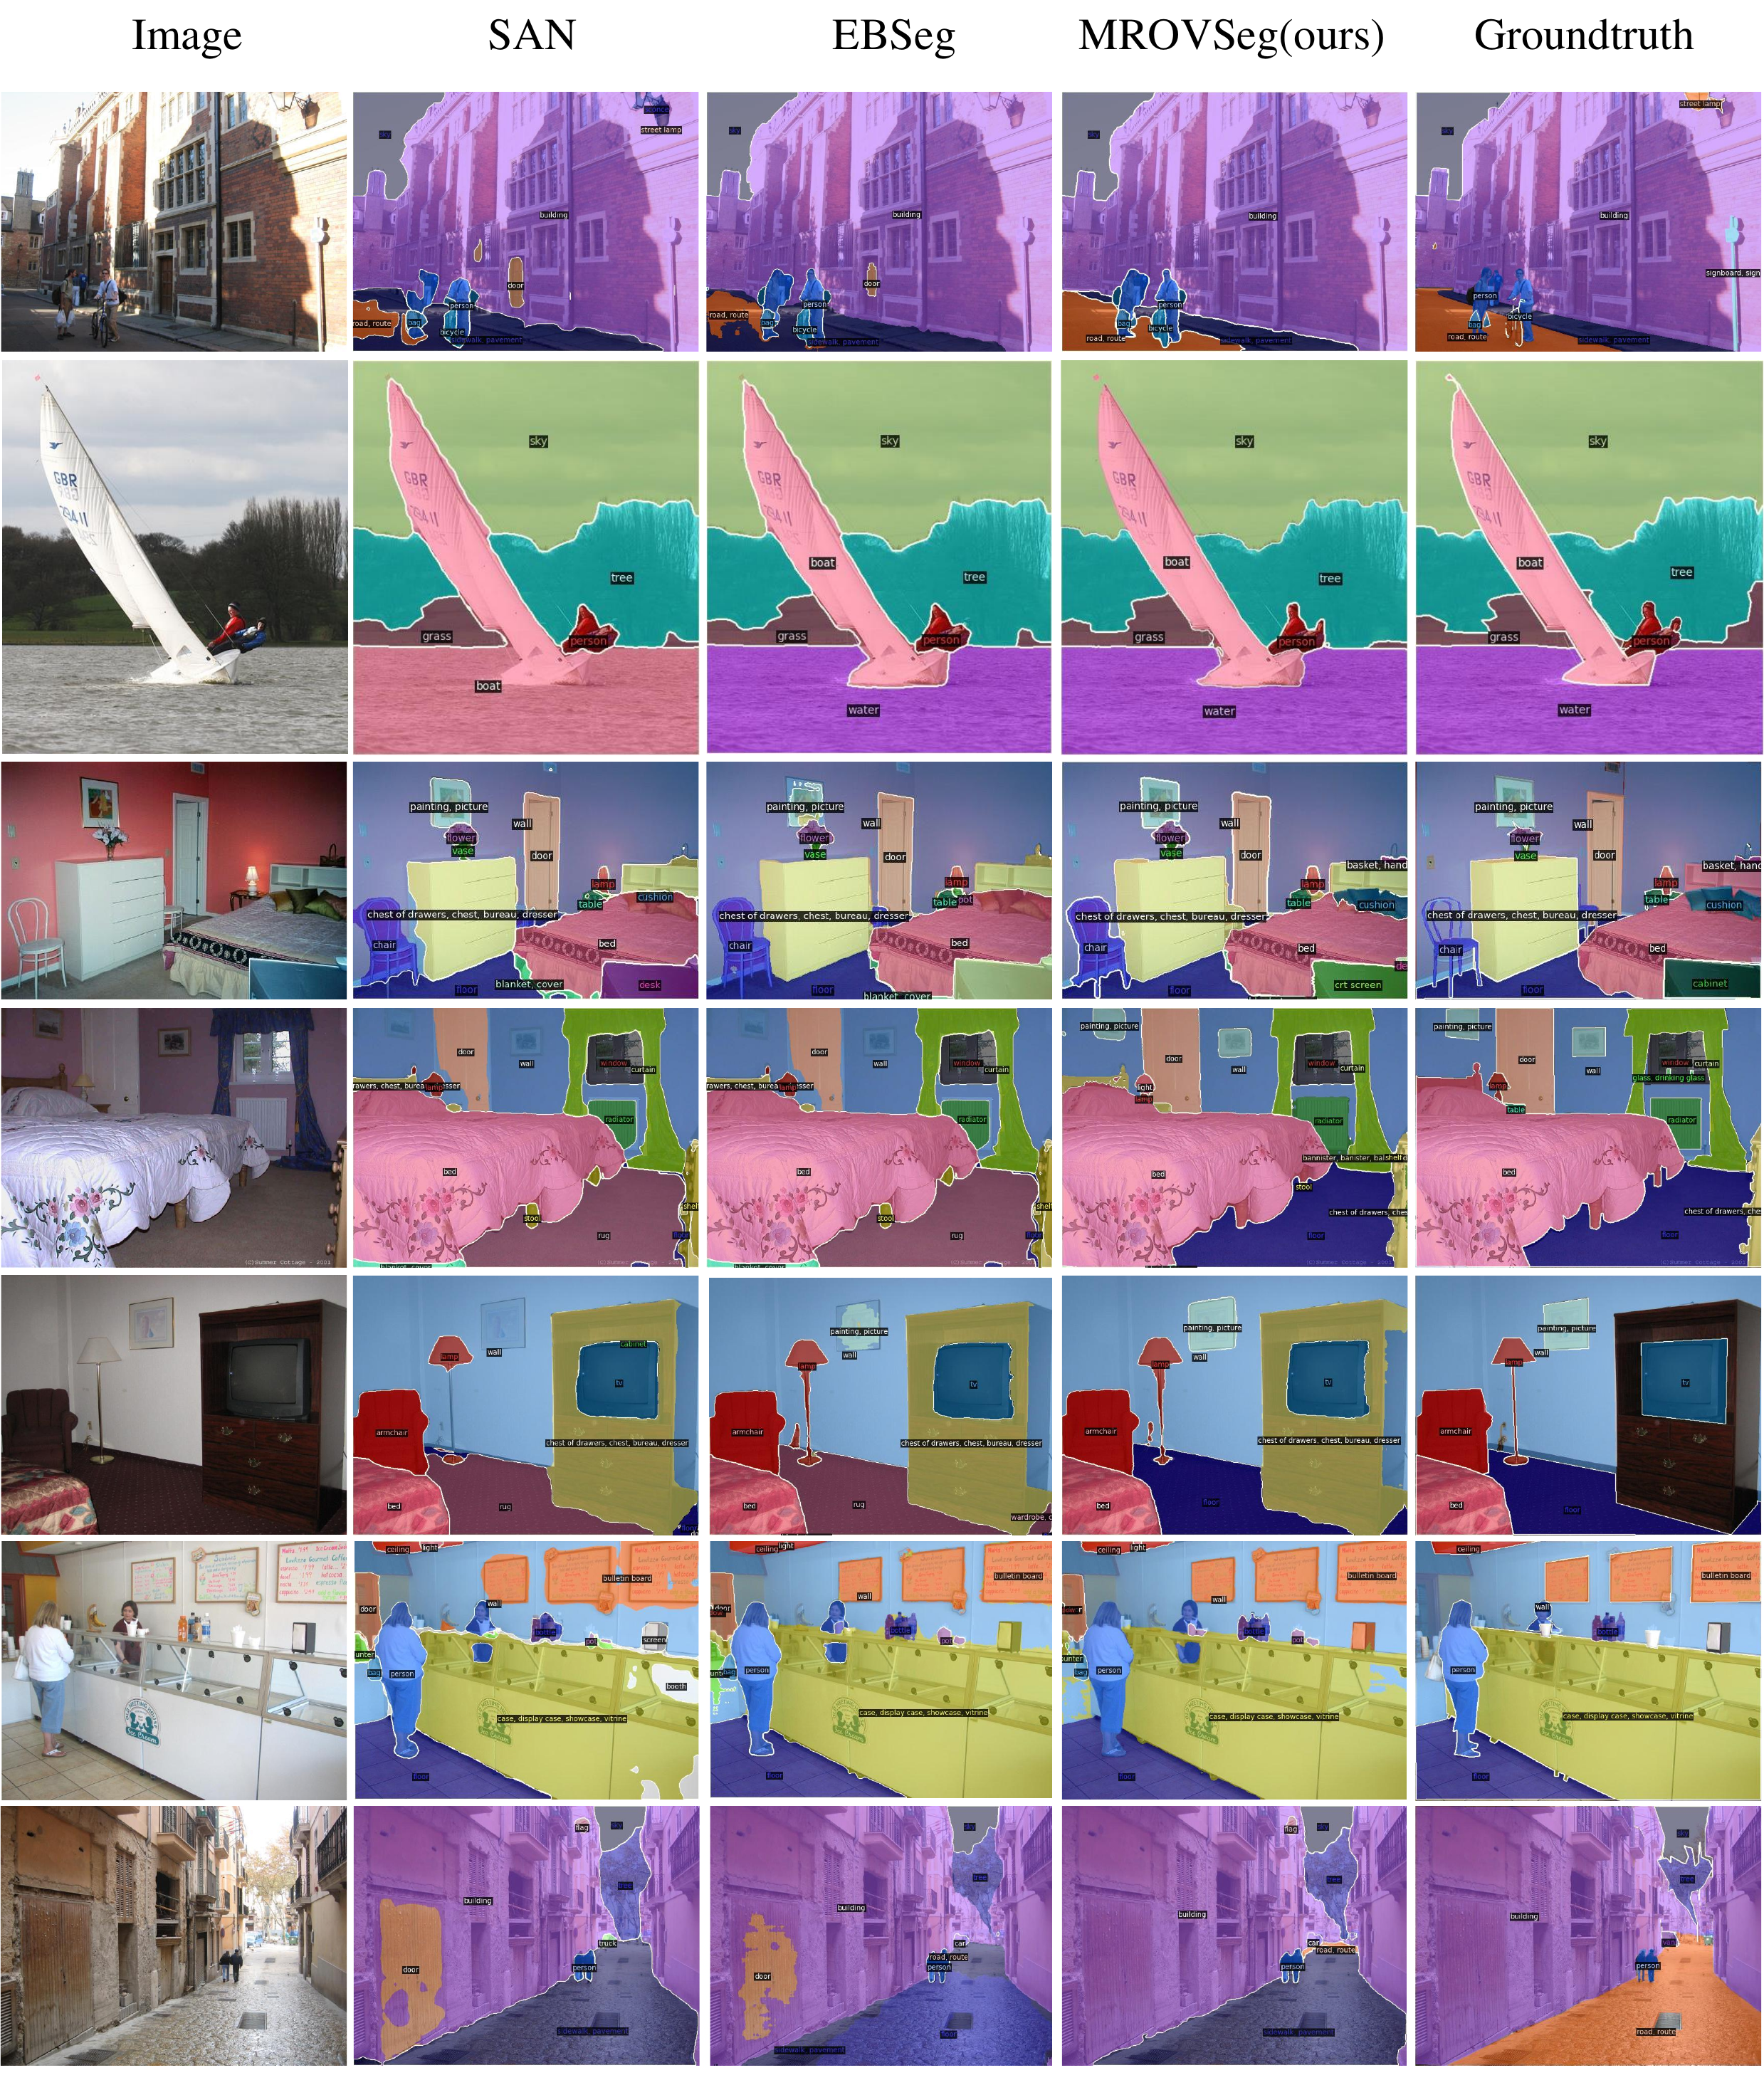}
    \caption{More Qualitative comparison with SAN~\cite{san} and EBSeg~\cite{ebseg}.}
    \label{fig:qualitative_coco}
  \hfill
\end{figure*}

\begin{figure*}[t]
  \centering
    % \fbox{\rule{0pt}{2in} \rule{.9\linewidth}{0pt}}
    \includegraphics[width=0.9\linewidth]{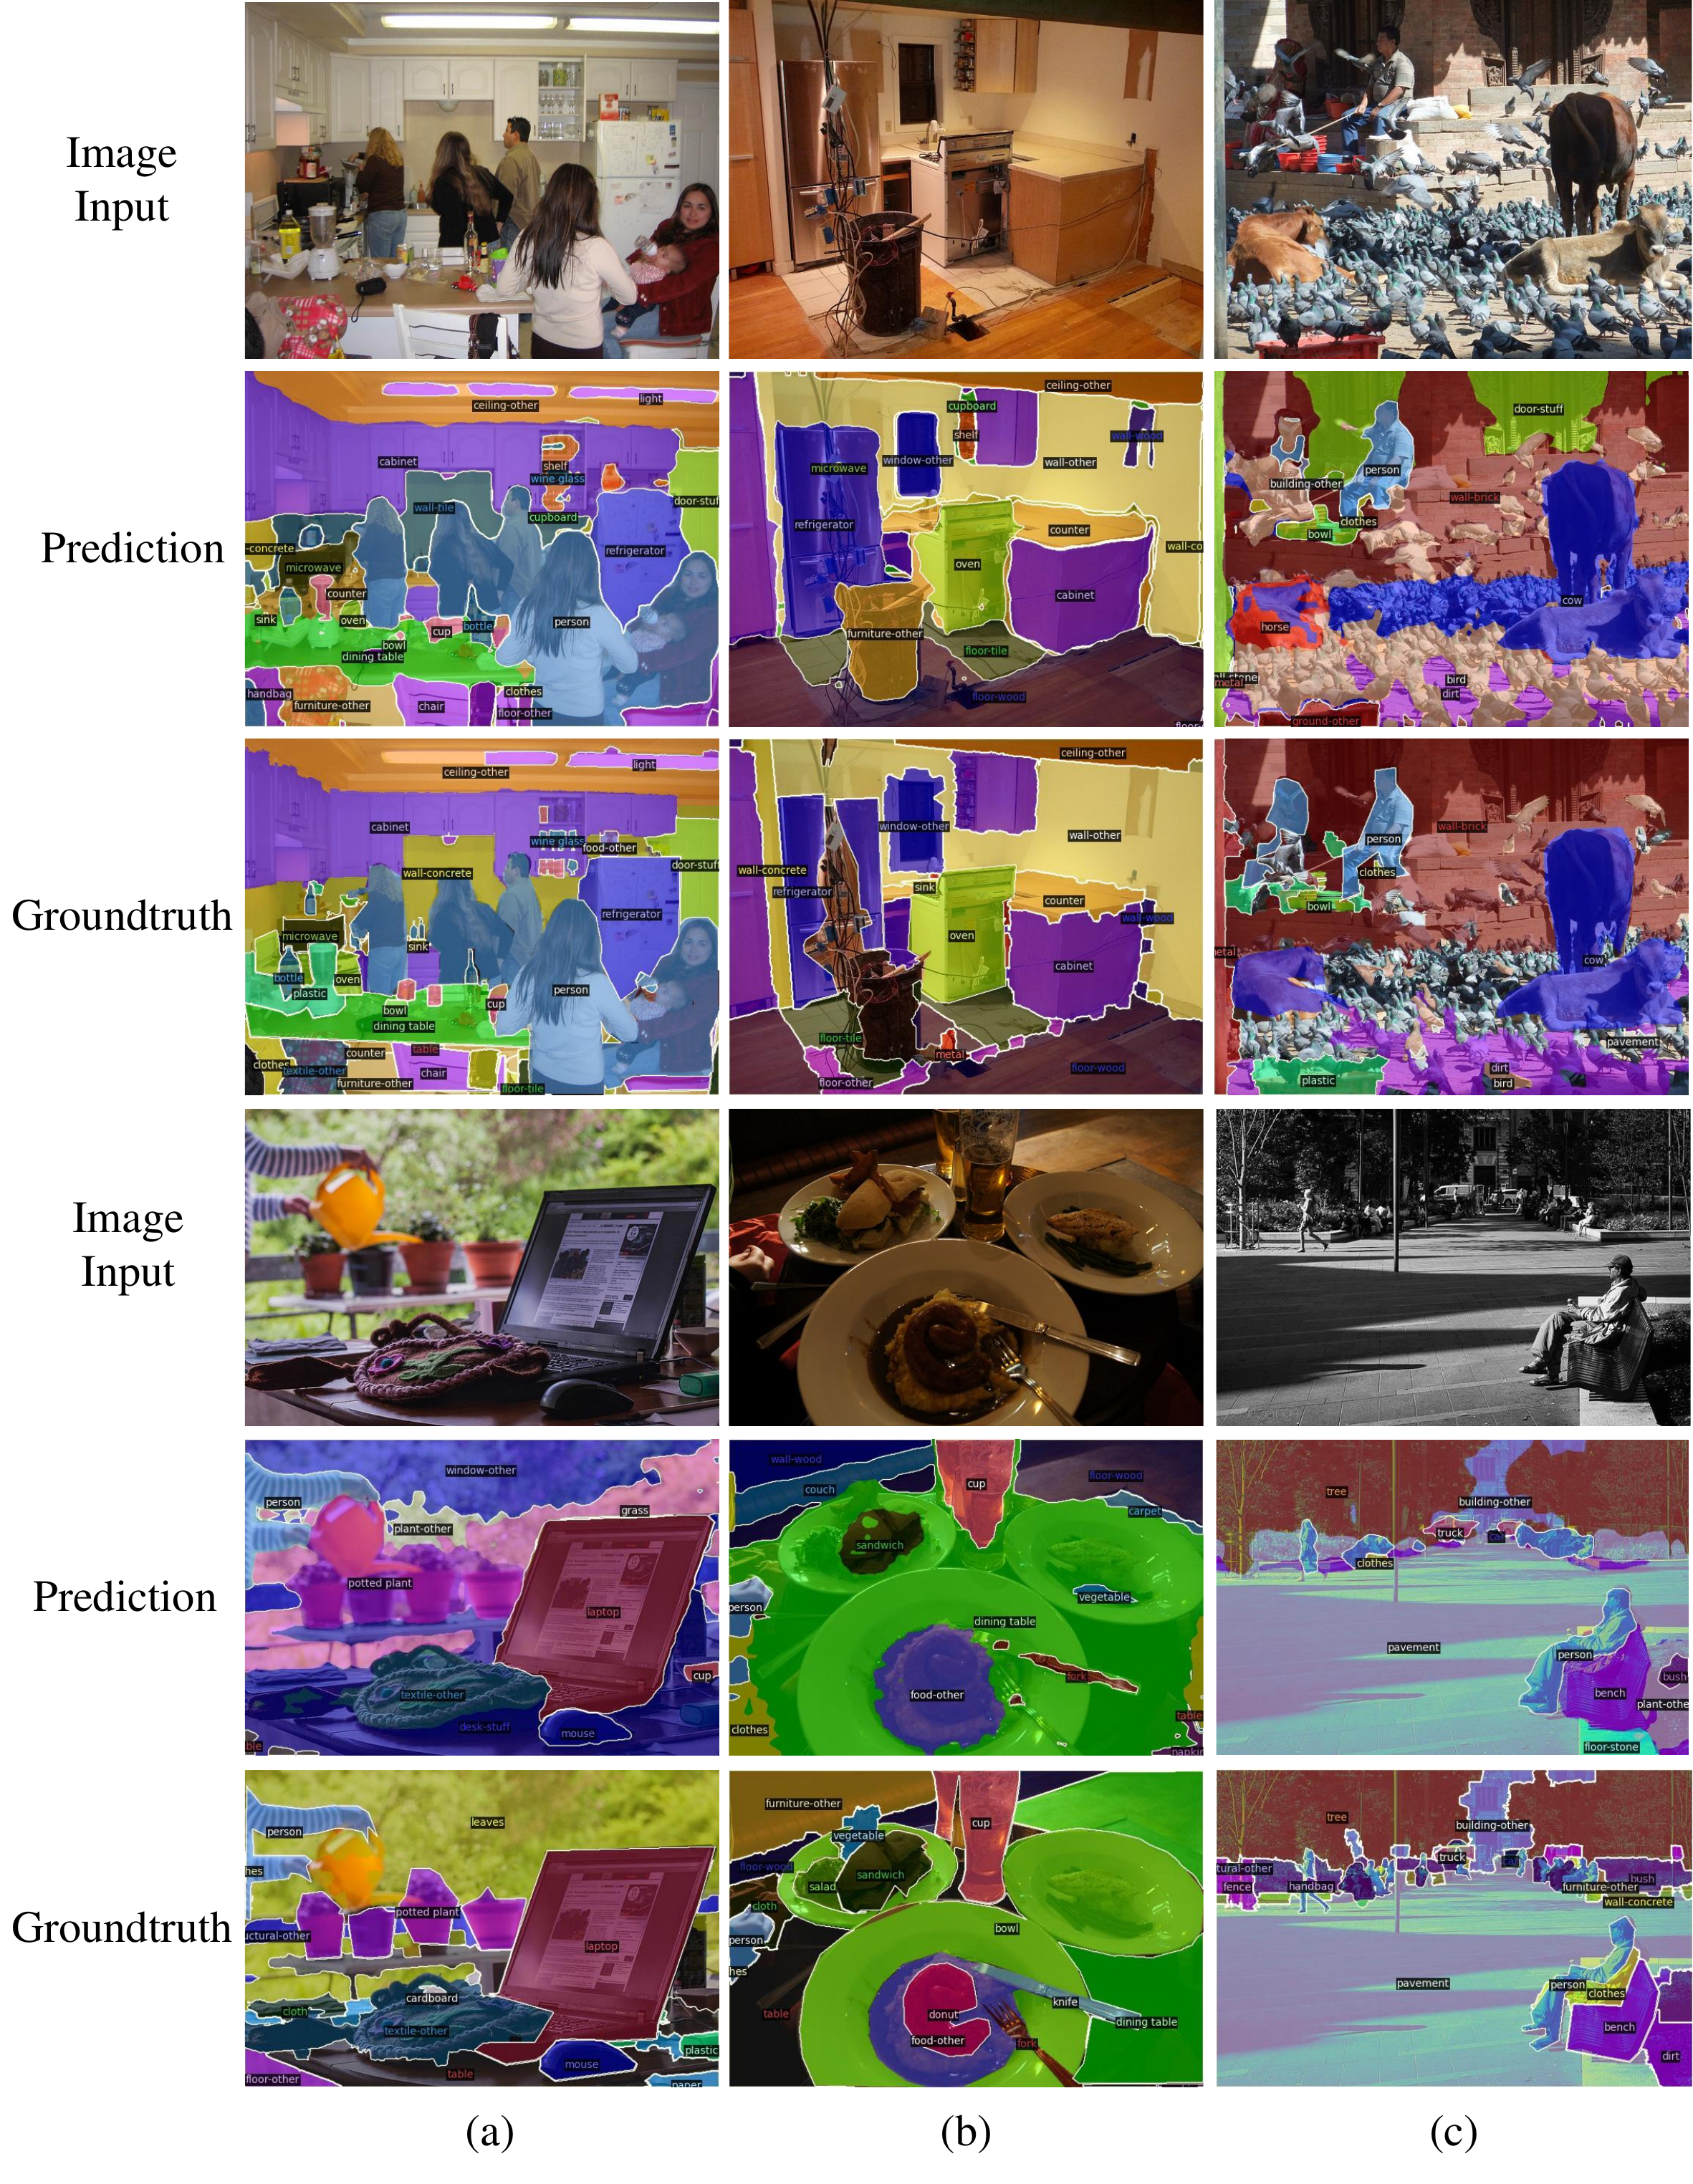}
    \caption{Qualitative results on COCO-Stuff~\cite{coco-stuff} \textit{val}. GT refer to groundtruth, Pred. refer to semantic prediction. We visualize the segmentation prediction of MROVSeg under complex real-world scenarios, such as muti-object scenes, low-light environment, and gray-scale photos.}
    \label{fig:qualitative_comparison}
  \hfill
\end{figure*}
\begin{figure*}[t]
  \centering
    % \fbox{\rule{0pt}{2in} \rule{.9\linewidth}{0pt}}
    \includegraphics[width=0.9\linewidth]{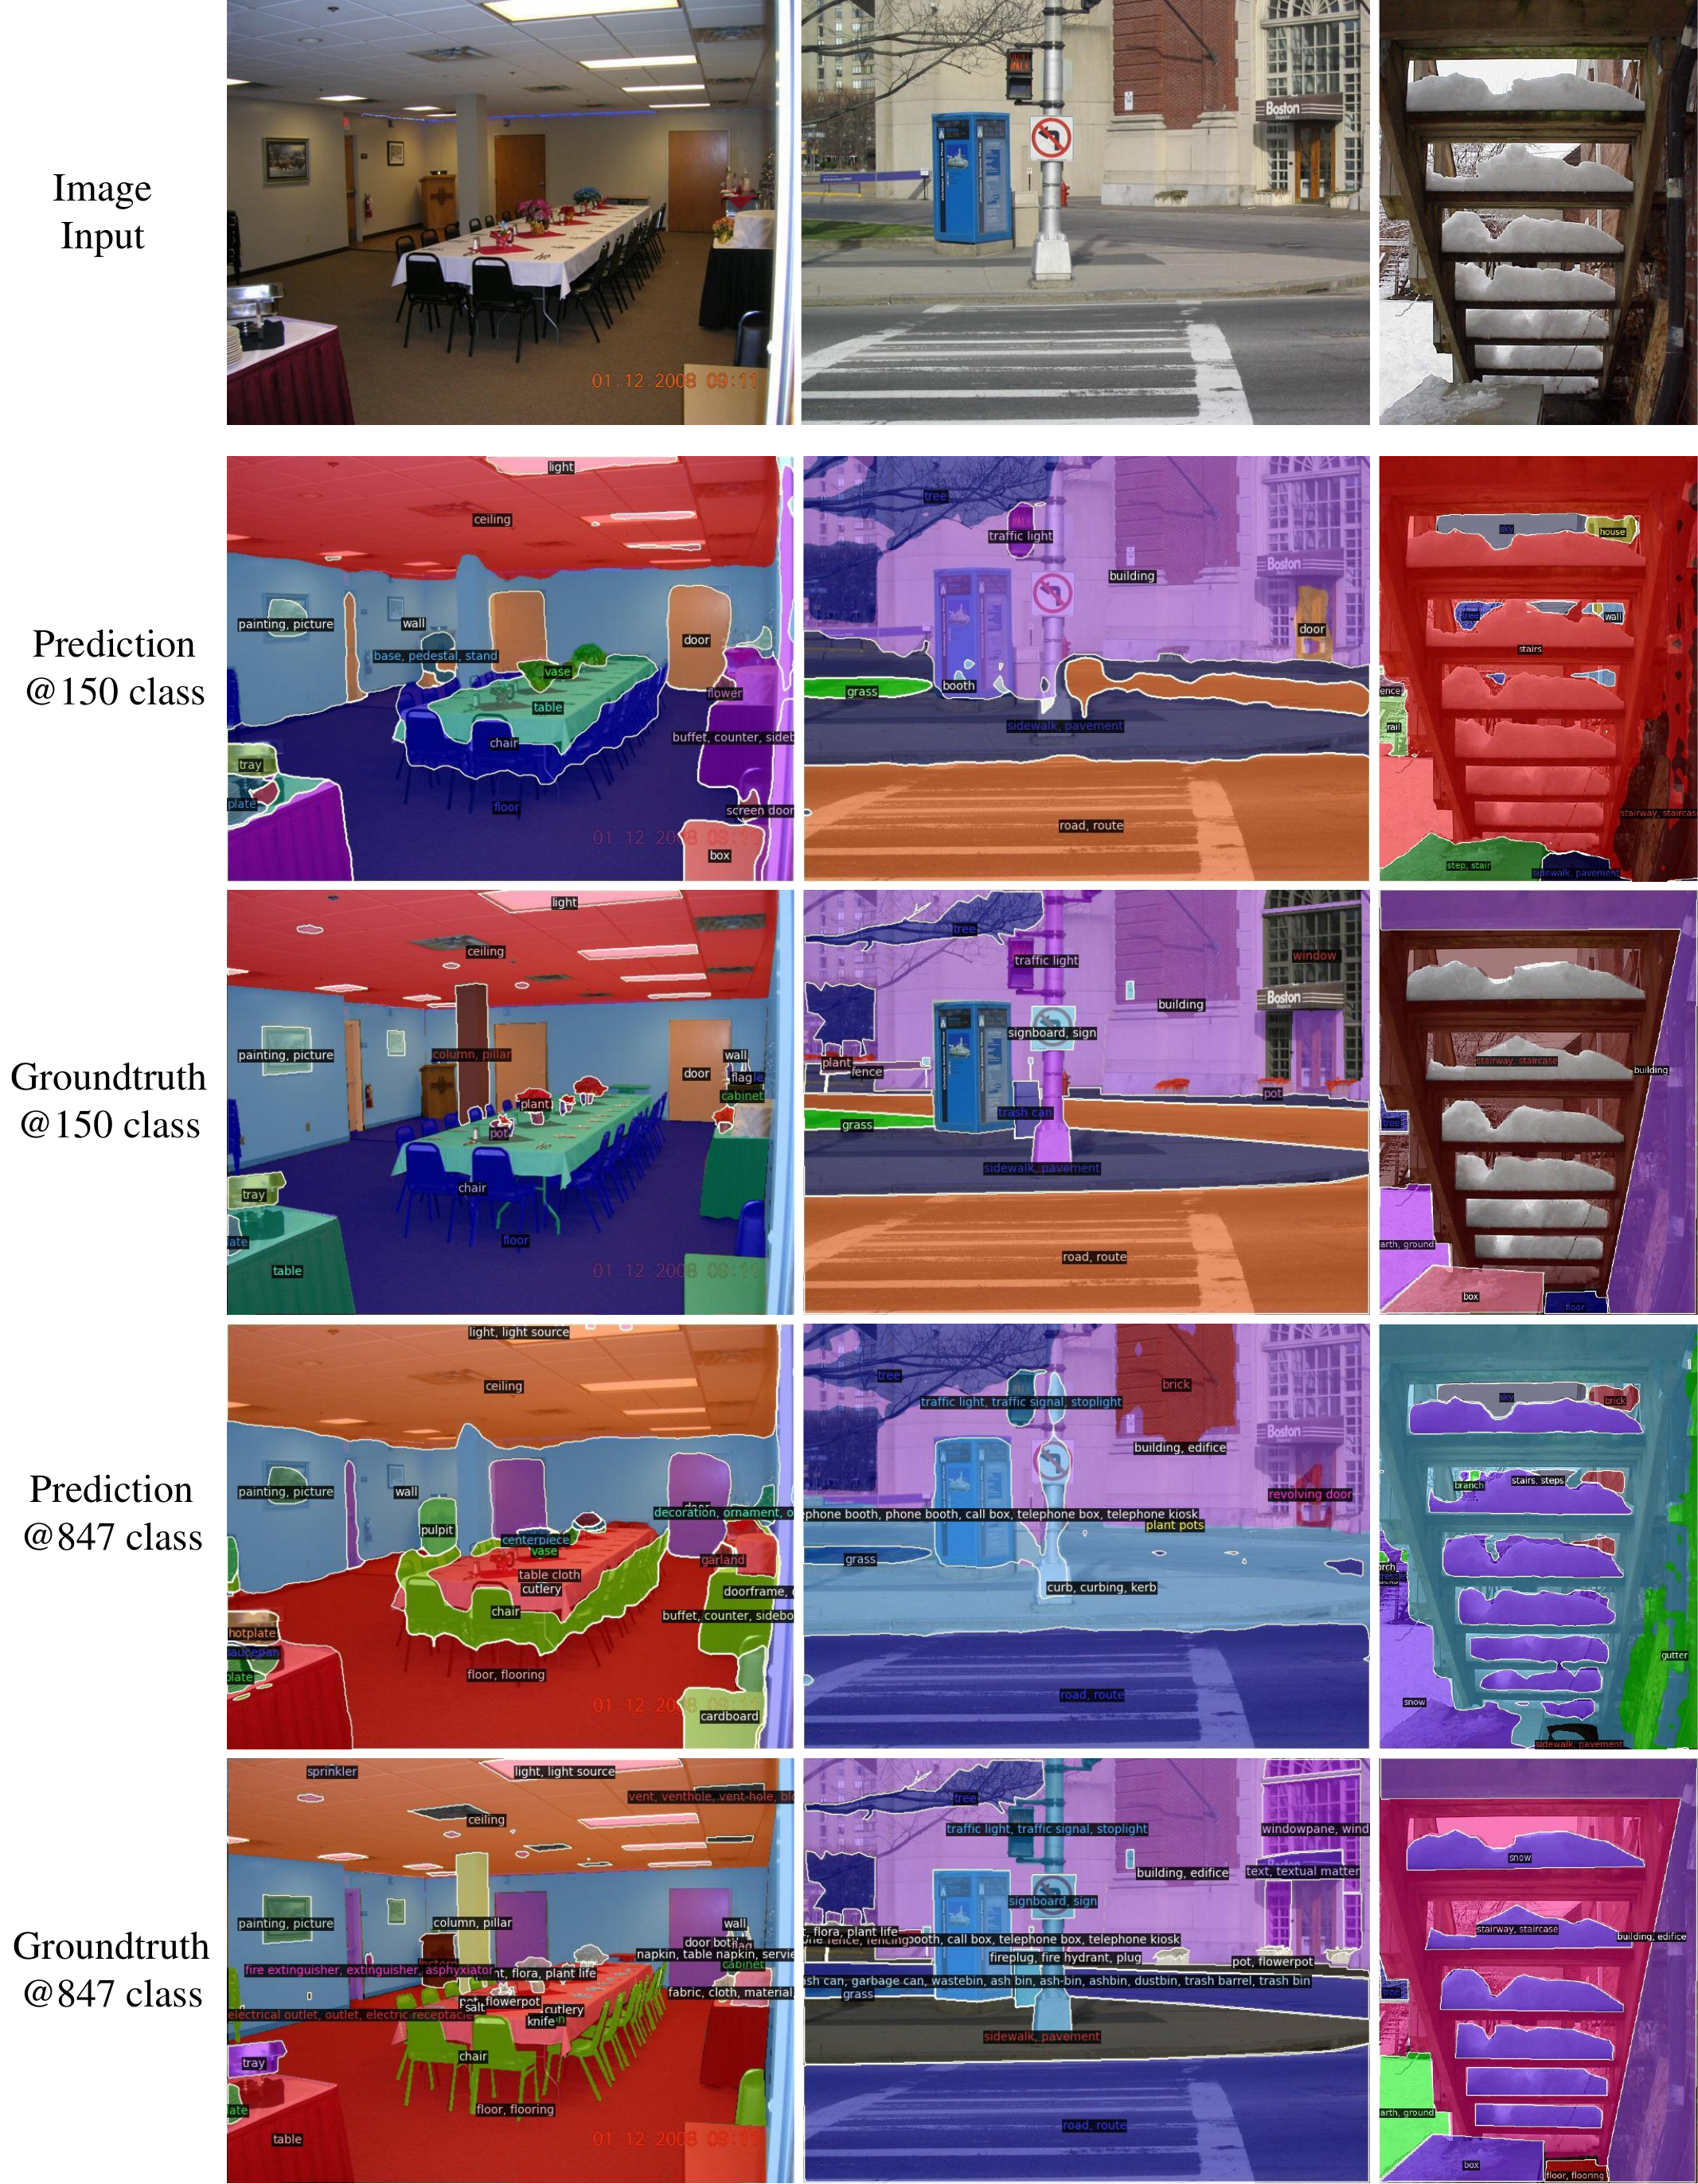}
    \caption{Qualitative results on ADE~\cite{ade} \textit{val}. Pred/GT-150/847 refer to the prediction/groundtruth for 150/847 semantic categories. We visualize the semantic prediction of a image on 150 and 847 categories.}
    \label{fig:qualitative_ade}
  \hfill
\end{figure*}
\begin{figure*}[t]
  \centering
    % \fbox{\rule{0pt}{2in} \rule{.9\linewidth}{0pt}}
    \includegraphics[width=1.0\linewidth]{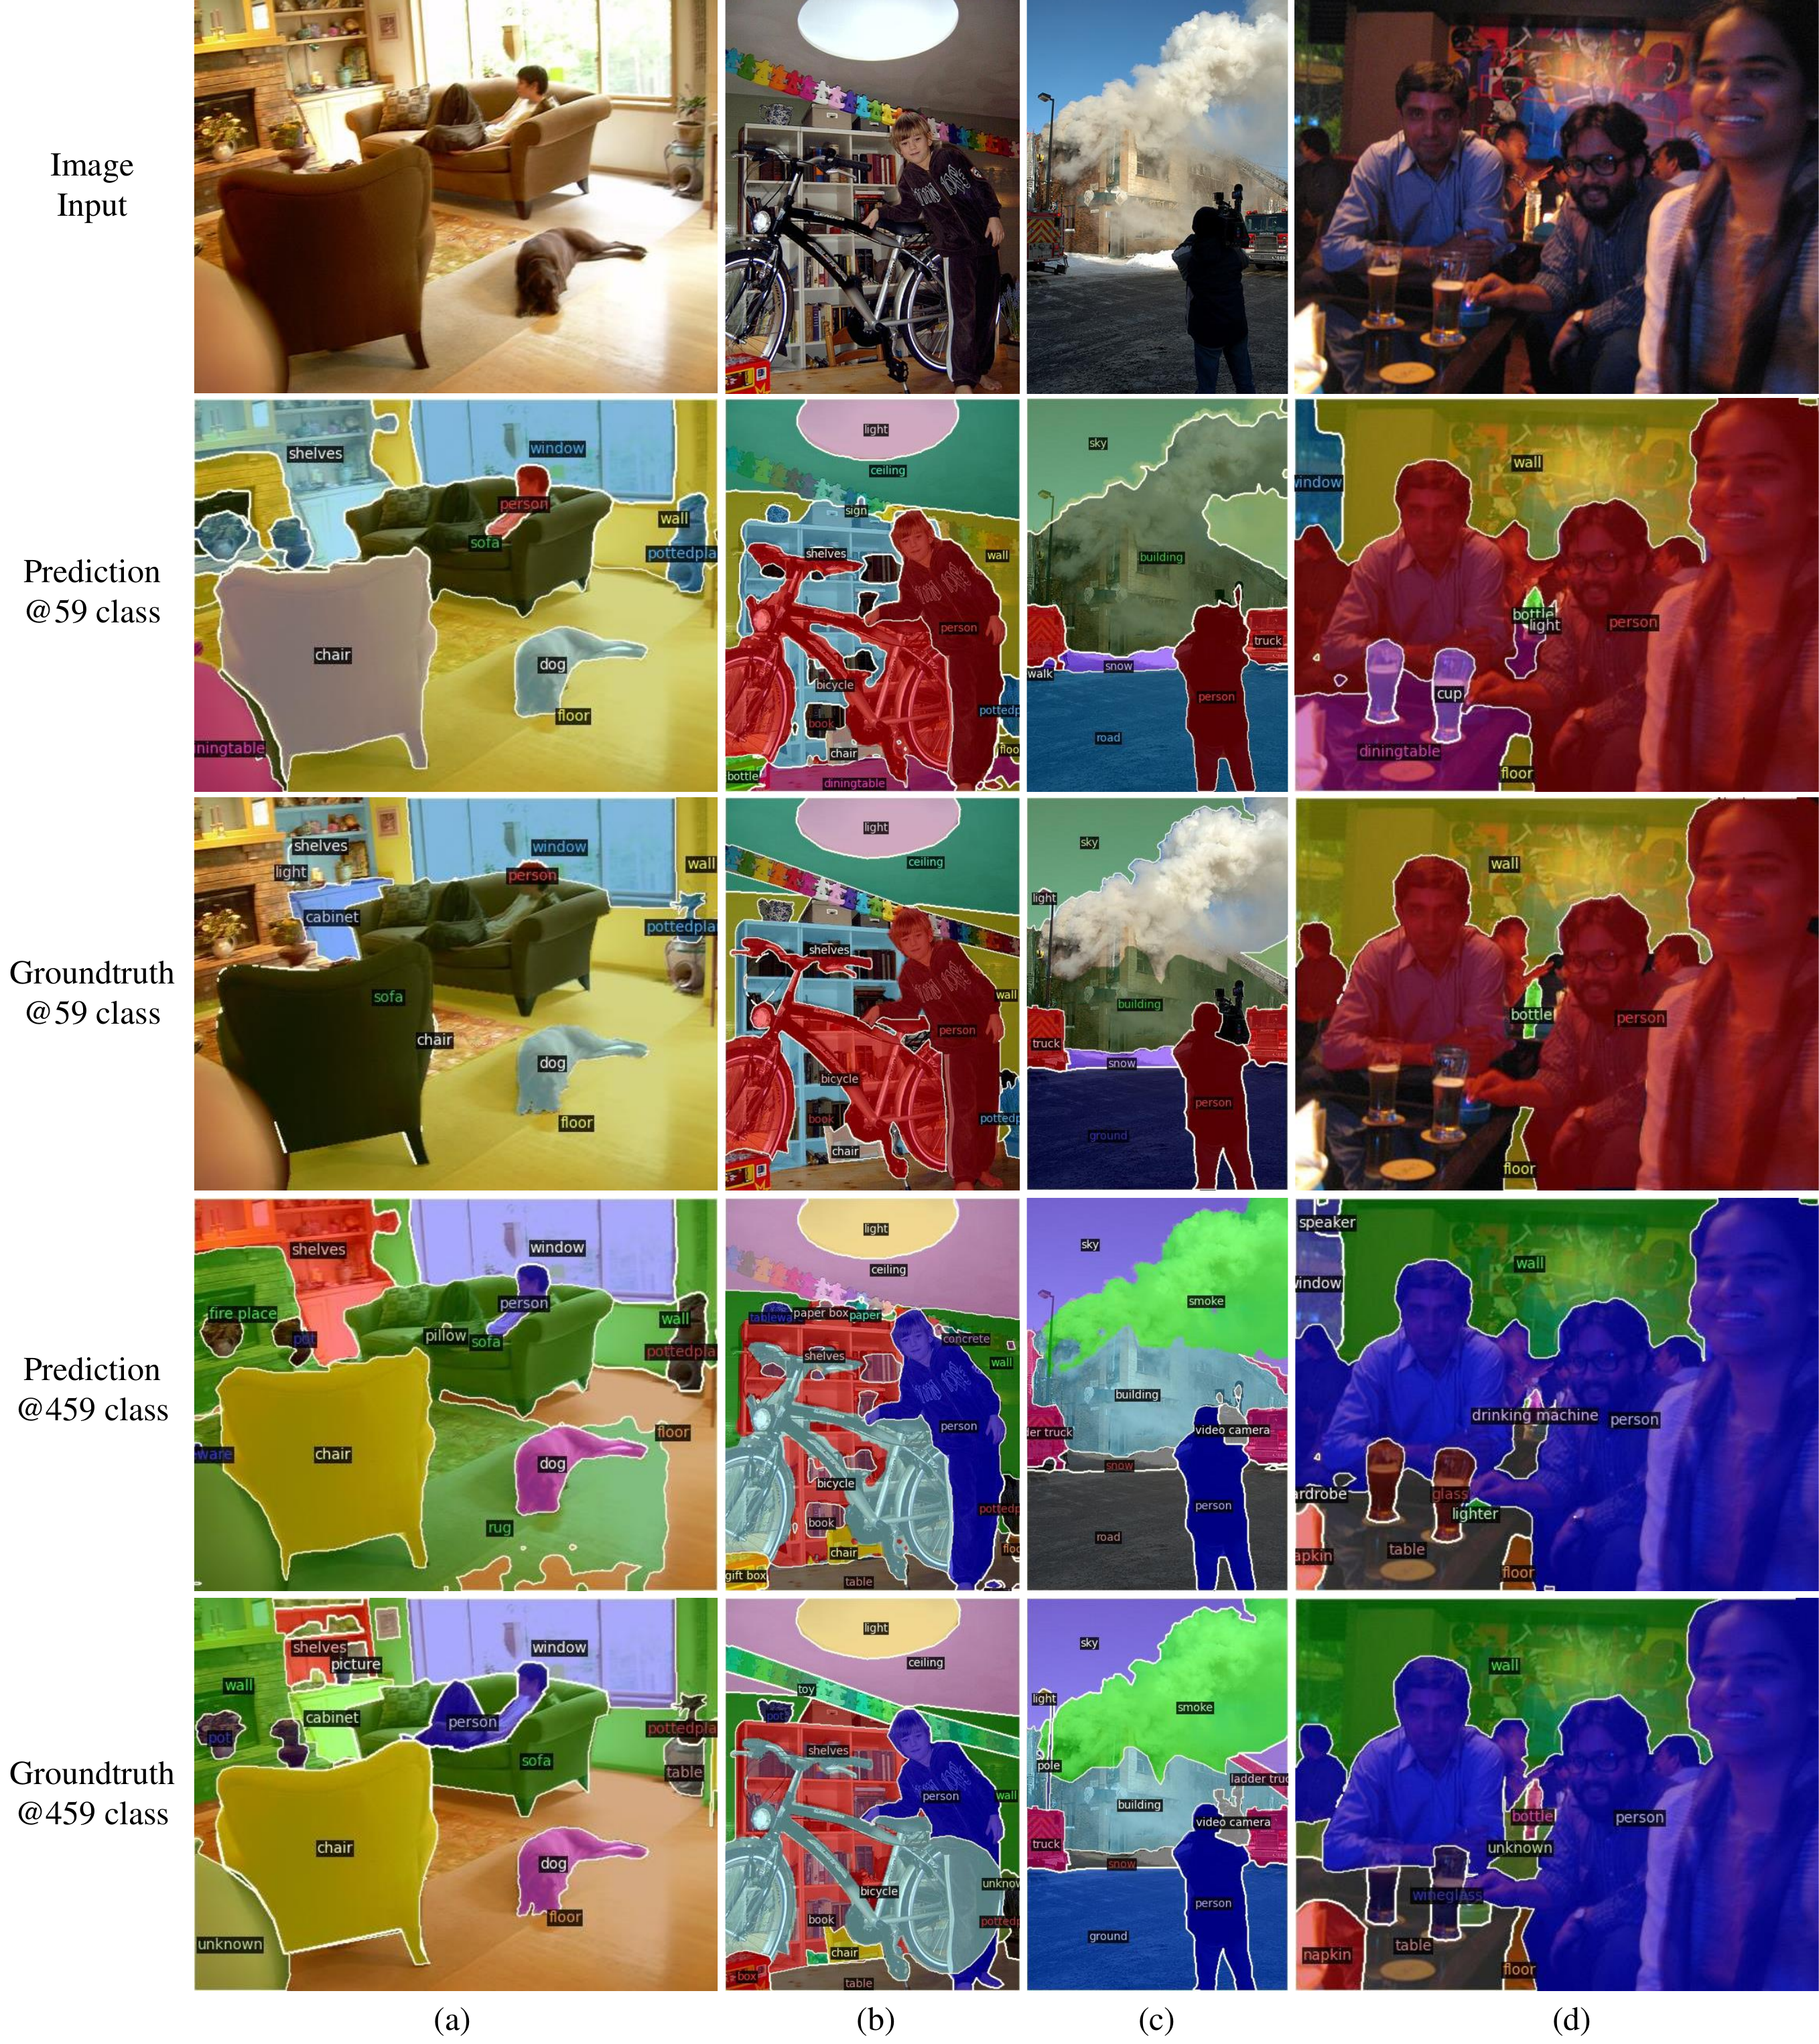}
    \caption{Qualitative results on Pascal Context~\cite{pc} \textit{val}. Similar to Fig.\ref{fig:qualitative_ade}, we visualize the prediction and groundtruth for 59 and 459 semantic categories respectively.}
    \label{fig:qualitative_pc}
  \hfill
\end{figure*}

\clearpage
